# Supplementary material for: Time-to-reach Bounds for Verification of Dynamical Systems Using the Koopman Spectrum
Source: arXiv:2411.05554 source file (2025-11-28)
Supplement: Supplementary file 1 [file appendix.tex]

\section*{Appendix}

\begin{table}[htbp]
        \centering
        \aboverulesep = 0pt \belowrulesep = 0pt
        \begin{adjustbox}
            {width=0.48\textwidth,center,keepaspectratio}
            \begin{tabular}{|M{0.02\textwidth}|M{0.4\textwidth}|}
                \toprule
                % \rowcolor[gray]{.90} 
                $S_{0}$ & $[-0.8, -0.7] \times [1.3, 1.39]$ \\
                \midrule
                $S_{1}$ & $[0.7, 0.8] \times [0.178, 0.3]$ \\
                \bottomrule
            \end{tabular}
        \end{adjustbox}
        \caption{Set definitions.}
\end{table}

\subsection{Proof of Theorem 1}

\begin{proof}
    Let $x_{0}$ be some point in $X_{0}$ such that $s_{T}(x_{0})\in X_{F}$ for some
    $T>0$. By definition, for any scalar-valued Koopman eigenfunction $\psi(x)$,
    its module of $x_{0}\in X_{0}$ at time $T$, which is $|e^{\lambda T}\psi(x_{0}
    )| = e^{\Real{(\lambda)T}}| \psi(x_{0})|$, should be between the minimum and
    maximum of the Koopman eigenfunction on $X_{F}$, that is,
    \begin{equation}
        \inf |\psi(X_{F})| \leq e^{\Real{(\lambda)T}}| \psi(x_{0})| \leq \sup |\psi
        (X_{F})|
    \end{equation}
    where
    $\inf |\psi(X_{0})| \leq | \psi(x_{0})| \leq \sup |\psi(X_{0})|, \forall x_{0}
    \in X_{0}$. This implies that for any feasible $T>0$, it should satisfy
    separately
    \begin{eqnarray*}
        \inf |\psi(X_F)| \leq e^{\Real{(\lambda)}T} \inf |\psi(X_0)| \leq e^{\Real{(\lambda)}T}
        \sup |\psi(X_0)| \\ e^{\Real{(\lambda)}T} \inf |\psi(X_0)| \leq e^{\Real{(\lambda)}T}
        \sup |\psi(X_0)| \leq \sup |\psi(X_F)|
    \end{eqnarray*}, then we have a tightest estimation of $e^{\Real{(\lambda)}T}$
    as follows
    \begin{eqnarray*}
        e^{\Real{(\lambda)T}} & \geq
        \frac{\inf |\psi(X_{F})|}{\inf |\psi(X_{0})|} & \geq
        \frac{\inf |\psi(X_{F})|}{\sup |\psi(X_{0})|} \\ e^{\Real{(\lambda)T}} &
        \leq \frac{\sup |\psi(X_{F})|}{\sup |\psi(X_{0})|} & \leq \frac{\sup |\psi(X_{F})|}{\inf
        |\psi(X_{0})|} \\
    \end{eqnarray*}
    Thus
    \begin{eqnarray*}
        % & \frac{\inf |\psi(X_F)|}{\inf |\psi(X_0)|} \leq e^{\Real{(\lambda)T}} \leq \frac{\sup |\psi(X_F)|}{\sup |\psi(X_0)|} \\
        % \Rightarrow & \log{\frac{\inf |\psi(X_F)|}{\inf |\psi(X_0)|}} \leq \Real{(\lambda)} T \leq \log{\frac{\sup |\psi(X_F)|}{\sup |\psi(X_0)|}} \\
        & \frac{\inf |\psi(X_{F})|}{\sup |\psi(X_{0})|} \leq e^{\Real{(\lambda)T}}
        \leq \frac{\sup |\psi(X_{F})|}{\inf |\psi(X_{0})|} \\ \Rightarrow & \log{\frac{\inf |\psi(X_{F})|}{\sup |\psi(X_{0})|}}
        \leq \Real{(\lambda)} T \leq \log{\frac{\sup |\psi(X_{F})|}{\inf |\psi(X_{0})|}}
    \end{eqnarray*}

    Let
    \begin{eqnarray*}
        % \mathcal{L}_I^{\psi}{(X_0,X_F)} = \log{\frac{\inf |\psi(X_F)|}{\inf |\psi(X_0)|}} \\
        % \mathcal{L}_S^{\psi}{(X_0,X_F)} = \log{\frac{\sup |\psi(X_F)|}{\sup |\psi(X_0)|}}
        \mathcal{L}^{g}{(W,V)} = \log{\frac{\sup |g(V)|}{\inf |g(W)|}}
    \end{eqnarray*}, then we have
    \begin{align*}
        - \Lc^{\psi}(X_{F},X_{0}) \leq \Real{(\lambda)}T \leq \Lc^{\psi}(X_{0},X_{F})
    \end{align*}
    \begin{eqnarray*}
        -\frac{\mathcal{L}^{\psi}{(X_F,X_0)}}{\Real{(\lambda)}} \leq T \leq
        \frac{\mathcal{L}^{\psi}{(X_0,X_F)}}{\Real{(\lambda)}}, \text{ if } \Real{(\lambda)}>0
        \\ \frac{\mathcal{L}^{\psi}{(X_0,X_F)}}{\Real{(\lambda)}} \leq T \leq -\frac{\mathcal{L}^{\psi}{(X_F,X_0)}}{\Real{(\lambda)}},
        \text{ if } \Real{(\lambda)}<0
    \end{eqnarray*}
\end{proof}

By applying parameterization with principal eigenfunctions, we have
\begin{align*}
    \Lc^{\psi}(X_{0},X_{F}) & = \log \sup_{x \in X_F}|\psi(x)| - \log \inf_{x \in X_0}|\psi(x)|                                                  \\
                            & \leq \sum_{i=1}^{n}\alpha_{i}\sup_{x \in X_F}|\psi_{i}(x)| - \sum_{i=1}^{n}\alpha_{i}\inf_{x \in X_0}|\psi_{i}(x)| \\
                            & = \sum_{i=1}^{n}\alpha_{i}\Lc^{\psi_i}(X_{0},X_{F})
\end{align*}

\subsection{Proof of probabilistic guarantee via sampling}

\begin{proof}
    Consider estimating the lower/upper bound of a function $f$ on a set $S$ via
    sampling, we define
    \begin{align*}
        \underline{N}^{f}_{S,\epsilon} & = \{ x \in S | f(x) - \underline{f}(S) \leq \epsilon\} \\
        \overline{N}^{f}_{S,\epsilon}  & = \{ x \in S | \overline{f}(S) - f(x) \leq \epsilon\},
    \end{align*}
    where $\epsilon>0$. Let the probability of a point in $\underline{N}^{f}_{S,\epsilon}$
    and $\overline{N}^{f}_{S,\epsilon}$ denoted by $\underline{P}_{S,\epsilon}\in
    [0,1]$ and $\overline{P}_{S,\epsilon}\in [0,1]$.

    For $d$ i.i.d. samples, the probability of obtaining a good estimation of the
    lower/upper bound of a function $f$ on $S$ is given by
    \begin{align*}
        \mathbb{P}\{\tilde{\underline{f}}(S) - \underline{f}(S) \leq \epsilon \} & = 1 - (1 - \underline{P}_{S,\epsilon})^{d} \\
        \mathbb{P}\{ \overline{f}(S)- \tilde{\overline{f}}(S) \leq \epsilon \}   & = 1 - (1 - \overline{P}_{S,\epsilon})^{d}  \\
    \end{align*}

    Since with enough samples when estimating the lower/upper bounds of function
    $g$ on the set $S$, we can have
    \begin{eqnarray*}
        0 \leq & \log \sup_{x \in S} |g(x)| - \log \sup_{x \in S} |\tilde{g}(x)|
        & \leq \frac{\epsilon}{2} \\ 0 \leq & \log \inf_{x \in S} |\tilde{g}(x)|
        - \log \inf_{x \in S} |g(x)| & \leq \frac{\epsilon}{2}
    \end{eqnarray*}
    then for each principal eigenfunction $\psi_{i}$, we can have
    \begin{align*}
        \Lc^{\tilde{\psi_i}}(X_{0},X_{F}) & = \log \sup_{x \in X_F}|\tilde{\psi_i}(x)| - \log \inf_{x \in X_0}|\tilde{\psi_i}(x)|                                 \\
                                          & \geq \log \sup_{x \in X_F}|\psi_{i}(x)| - \frac{\epsilon}{2}- \log \inf_{x \in X_0}|\psi_{i}(x)| - \frac{\epsilon}{2} \\
                                          & = \Lc^{\psi_i}(X_{0},X_{F}) - \epsilon                                                                                \\
        \Lc^{\tilde{\psi_i}}(X_{0},X_{F}) & = \log \sup_{x \in X_F}|\tilde{\psi_i}(x)| - \log \inf_{x \in X_0}|\tilde{\psi_i}(x)|                                 \\
                                          & \leq \log \sup_{x \in X_F}|\psi_{i}(x)| - \log \inf_{x \in X_0}|\psi_{i}(x)|                                          \\
                                          & = \Lc^{\psi_i}(X_{0},X_{F})
    \end{align*}

    This implies
    \begin{eqnarray*}
        % 0 \leq \Lc^{\psi_i}(X_0,X_F) - \Lc^{\tilde{\psi_i}}(X_0,X_F) \leq \epsilon
        \Lc^{\psi_i}(X_0,X_F) - \epsilon \leq \Lc^{\tilde{\psi_i}}(X_0,X_F) \leq
        \Lc^{\psi_i}(X_0,X_F) \\ - \Lc^{\psi_i}(X_F,X_0) \leq -\Lc^{\tilde{\psi_i}}(X_F,X_0)
        \leq -\Lc^{\psi_i}(X_F,X_0) + \epsilon \\
        % \sum_{i=1}^n \alpha_i [\Lc^{\psi_i}(X_0,X_F) - \epsilon ] &\leq \sum_{i=1}^n \alpha_i \Lc^{\tilde{\psi_i}}(X_0,X_F) \\ &
        % \leq \sum_{i=1}^n \alpha_i \Lc^{\psi_i}(X_0,X_F)
    \end{eqnarray*}

    if $\Real{(\lambda)}= \sum_{i=1}^{n}\Real{(\lambda_i)}>0$, for the upper bound
    \begin{align*}
        \tilde{\overline{I}} & = \frac{\sum_{i=1}^{n}\alpha_{i}\Lc^{\tilde{\psi_i}}(X_{0},X_{F})}{\sum_{i=1}^{n}\alpha_{i}\Real{(\lambda_i)}}          \\
                             & \leq \frac{\sum_{i=1}^{n}\alpha_{i}\Lc^{\psi_i}(X_{0},X_{F})}{\sum_{i=1}^{n}\alpha_{i}\Real{(\lambda_i)}}= \overline{I} \\
        \tilde{\overline{I}} & = \frac{\sum_{i=1}^{n}\alpha_{i}\Lc^{\tilde{\psi_i}}(X_{0},X_{F})}{\sum_{i=1}^{n}\alpha_{i}\Real{(\lambda_i)}}          \\
                             & \geq \frac{\sum_{i=1}^{n}\alpha_{i}[\Lc^{\psi_i}(X_{0},X_{F}) - \epsilon] }{\sum_{i=1}^{n}\alpha_{i}\Real{(\lambda_i)}} \\
                             & = \overline{I}- \frac{\sum_{i=1}^{n}\alpha_{i}\epsilon}{\sum_{i=1}^{n}\alpha_{i}\Real{(\lambda_i)}}
    \end{align*}
    for the lower bound
    \begin{align*}
        \tilde{\underline{I}} & = - \frac{\sum_{i=1}^{n}\alpha_{i}\Lc^{\tilde{\psi_i}}(X_{F},X_{0})}{\sum_{i=1}^{n}\alpha_{i}\Real{(\lambda_i)}}           \\
                              & \leq \frac{\sum_{i=1}^{n}\alpha_{i}[- \Lc^{\psi_i}(X_{F},X_{0}) + \epsilon] }{\sum_{i=1}^{n}\alpha_{i}\Real{(\lambda_i)}}  \\
                              & = \underline{I}+ \frac{\sum_{i=1}^{n}\alpha_{i}\epsilon}{\sum_{i=1}^{n}\alpha_{i}\Real{(\lambda_i)}}                       \\
        \tilde{\underline{I}} & = - \frac{\sum_{i=1}^{n}\alpha_{i}\Lc^{\tilde{\psi_i}}(X_{F},X_{0})}{\sum_{i=1}^{n}\alpha_{i}\Real{(\lambda_i)}}           \\
                              & \geq - \frac{\sum_{i=1}^{n}\alpha_{i}\Lc^{\psi_i}(X_{F},X_{0})}{\sum_{i=1}^{n}\alpha_{i}\Real{(\lambda_i)}}= \underline{I}
    \end{align*}

    if $\Real{(\lambda)}= \sum_{i=1}^{n}\Real{(\lambda_i)}<0$, for the upper bound
    \begin{align*}
        \tilde{\overline{I}} & = - \frac{\sum_{i=1}^{n}\alpha_{i}\Lc^{\tilde{\psi_i}}(X_{F},X_{0})}{\sum_{i=1}^{n}\alpha_{i}\Real{(\lambda_i)}}                                                                                 \\
                             & \leq - \frac{\sum_{i=1}^{n}\alpha_{i}\Lc^{\psi_i}(X_{F},X_{0})}{\sum_{i=1}^{n}\alpha_{i}\Real{(\lambda_i)}}= \overline{I}                                                                        \\
        \tilde{\overline{I}} & = - \frac{\sum_{i=1}^{n}\alpha_{i}\Lc^{\tilde{\psi_i}}(X_{F},X_{0})}{\sum_{i=1}^{n}\alpha_{i}\Real{(\lambda_i)}}                                                                                 \\
                             & \geq - \frac{\sum_{i=1}^{n}\alpha_{i}\Lc^{\psi_i}(X_{0},X_{F})}{\sum_{i=1}^{n}\alpha_{i}\Real{(\lambda_i)}}+ \frac{\sum_{i=1}^{n}\alpha_{i}\epsilon}{\sum_{i=1}^{n}\alpha_{i}\Real{(\lambda_i)}} \\
                             & = \overline{I}+ \frac{\sum_{i=1}^{n}\alpha_{i}\epsilon}{\sum_{i=1}^{n}\alpha_{i}\Real{(\lambda_i)}}
    \end{align*}
    for the lower bound
    \begin{align*}
        \tilde{\underline{I}} & = \frac{\sum_{i=1}^{n}\alpha_{i}\Lc^{\tilde{\psi_i}}(X_{0},X_{F})}{\sum_{i=1}^{n}\alpha_{i}\Real{(\lambda_i)}}                                                                                 \\
                              & \leq \frac{\sum_{i=1}^{n}\alpha_{i}\Lc^{\psi_i}(X_{0},X_{F})}{\sum_{i=1}^{n}\alpha_{i}\Real{(\lambda_i)}}- \frac{\sum_{i=1}^{n}\alpha_{i}\epsilon}{\sum_{i=1}^{n}\alpha_{i}\Real{(\lambda_i)}} \\
                              & = \underline{I}- \frac{\sum_{i=1}^{n}\alpha_{i}\epsilon}{\sum_{i=1}^{n}\alpha_{i}\Real{(\lambda_i)}}                                                                                           \\
        \tilde{\underline{I}} & = \frac{\sum_{i=1}^{n}\alpha_{i}\Lc^{\tilde{\psi_i}}(X_{0},X_{F})}{\sum_{i=1}^{n}\alpha_{i}\Real{(\lambda_i)}}                                                                                 \\
                              & \geq \frac{\sum_{i=1}^{n}\alpha_{i}\Lc^{\psi_i}(X_{0},X_{F})}{\sum_{i=1}^{n}\alpha_{i}\Real{(\lambda_i)}}= \underline{I}
    \end{align*}

    Thus
    \begin{align*}
        \text{if } & \Real{(\lambda)}>0                                                                                                                                                                                                                                                                      \\
                   & \tilde{\underline{I}}\in [\underline{I}, \underline{I}+ \frac{\sum_{i=1}^{n}\alpha_{i}\epsilon}{\sum_{i=1}^{n}\alpha_{i}\Real{(\lambda_i)}}], \tilde{\overline{I}}\in [\overline{I}- \frac{\sum_{i=1}^{n}\alpha_{i}\epsilon}{\sum_{i=1}^{n}\alpha_{i}\Real{(\lambda_i)}}, \overline{I}] \\
        \text{if } & \Real{(\lambda)}<0                                                                                                                                                                                                                                                                      \\
                   & \tilde{\underline{I}}\in [\underline{I}, \underline{I}- \frac{\sum_{i=1}^{n}\alpha_{i}\epsilon}{\sum_{i=1}^{n}\alpha_{i}\Real{(\lambda_i)}}], \tilde{\overline{I}}\in [\overline{I}+ \frac{\sum_{i=1}^{n}\alpha_{i}\epsilon}{\sum_{i=1}^{n}\alpha_{i}\Real{(\lambda_i)}}, \overline{I}]
    \end{align*}
    which means the obtained reach time bound via sampling always a subset of
    the exact reach time bound such that $\tilde{I}\subseteq I$, even though the
    exact reach time bound parameterized by the principal eigen pairs is still an
    over-approximation of the true reach time bound. Additionally, we can also conclude
    that the Hausdorff distance distance between $\tilde{I}$ and $I$ satisfy
    \begin{align*}
        d_{H}(\tilde{I},I) & \leq \max \{ \frac{\epsilon \sum_{i=1}^{n} \alpha_{i}}{ \sum_{i=1}^{n} \alpha_{i} |\Real{(\lambda_i)|}}, \forall \alpha_{i} \in [0,+\infty), i=1, \cdots, n \} \\
                           & \leq \frac{\epsilon}{|\Real{(\lambda_i)}|_{\min}}
    \end{align*}

    Since obtaining a good estimation ($\epsilon$ close to the exact bound) via
    sampling for the bounds of each $\psi_{i}$ on $X_{0}$ and $X_{F}$ such that
    \begin{align*}
        0 \leq \log \sup_{x \in X_0}|\psi_{i}(x)| - \log \sup_{x \in X_0}|\tilde{\psi_i}(x)| \leq \frac{\epsilon}{2} \\
        0 \leq \log \inf_{x \in X_0}|\tilde{\psi_i}(x)| - \log \inf_{x \in X_0}|\psi_{i}(x)| \leq \frac{\epsilon}{2} \\
        0 \leq \log \sup_{x \in X_F}|\psi_{i}(x)| - \log \sup_{x \in X_F}|\tilde{\psi_i}(x)| \leq \frac{\epsilon}{2} \\
        0 \leq \log \inf_{x \in X_F}|\tilde{\psi_i}(x)| - \log \inf_{x \in X_F}|\psi_{i}(x)| \leq \frac{\epsilon}{2} \\
    \end{align*}
    is just one sufficient condition to guarantee the bounded Hausdorff distance
    with sampling. Thus
    \begin{align*}
        \mathbb{P}\left\{ d_{H} (\tilde{I},I) \leq \frac{\epsilon}{|\Real{(\lambda_i)}|_{\min}}\right\} & \geq \mathbb{P}\left( \bigcap_{i=1}^{n} E_{i} \right)     \\
                                                                                                        & = 1- \mathbb{P}\left( \bigcup_{i=1}^{n} E_{i}^{c} \right) \\
                                                                                                        & \geq 1 - \sum_{i=1}^{n} \mathbb{P}(E_{i}^{c})
    \end{align*}
    where $E_{i}$ denotes the event that the estimated bounds of eigenfunction $\psi
    _{i}$ on $X_{0}$ and $X_{F}$ satisfy the above $\epsilon$ requirements when sampling,
    for i.i.d $n_{0}$ samples on $X_{0}$ and $n_{F}$ samples on $X_{F}$,
    \begin{align*}
        \mathbb{P}(E_{i})     & = (1 - \mathbb{P}_{\epsilon,X_0,\underline{\psi_i}}^{n_0}) (1 - \mathbb{P}_{\epsilon,X_0,\overline{\psi_i}}^{n_0}) (1 - \mathbb{P}_{\epsilon,X_F,\underline{\psi_i}}^{n_F}) (1 - \mathbb{P}_{\epsilon,X_F,\overline{\psi_i}}^{n_F}) \\
        \mathbb{P}(E_{i}^{c}) & = 1 - \mathbb{P}(E_{i})
    \end{align*}

    If $n_{0}$ and $n_{F}$ satisfy the following requirement
    \begin{align*}
        \sum_{i=1}^{n} \mathbb{P}(E_{i}^{c}) \leq \delta
    \end{align*}
    then for any $N_{0} \geq n_{0}$ and $N_{F} \geq n_{F}$, we have
    \begin{align*}
        \mathbb{P}\left\{ d_{H} (\tilde{I},I) \leq \frac{\epsilon}{|\Real{(\lambda_i)}|_{\min}}\right\} & \geq 1-\delta
    \end{align*}

\end{proof}

\subsection{Proof of Error Bounds with respect to eigen pair inaccuracy}

% In the case of inaccurate eigen pairs, i.e., $\hat{\psi}(x) = \psi(x)+\epsilon(x)$
